# Supplementary material for: Quantifying Spatial Under-reporting Disparities in Resident Crowdsourcing
Source: arXiv:2204.08620 source file (2023-12-06)
Supplement: Supplementary file 1 [file generalize_temporal.tex]

\subsection{Analyzing temporal reporting variation}
\label{app:generalize_temporal}

In this section, we present results from a \textbf{Temporal} analysis applied to both NYC and Chicago data. In this analysis, we include the \textit{Created Month} of each incident with the incident-level covariates (corresponding to the month of the first report for that incident). We use an AR(1) model for the prior of the month coefficients to model the dependencies. In such models, each month coefficient is assumed to be normally distributed with a mean equal to the coefficient of the previous month.

\begin{figure}[tb]
	\centering
	\includegraphics[width = .8\textwidth]{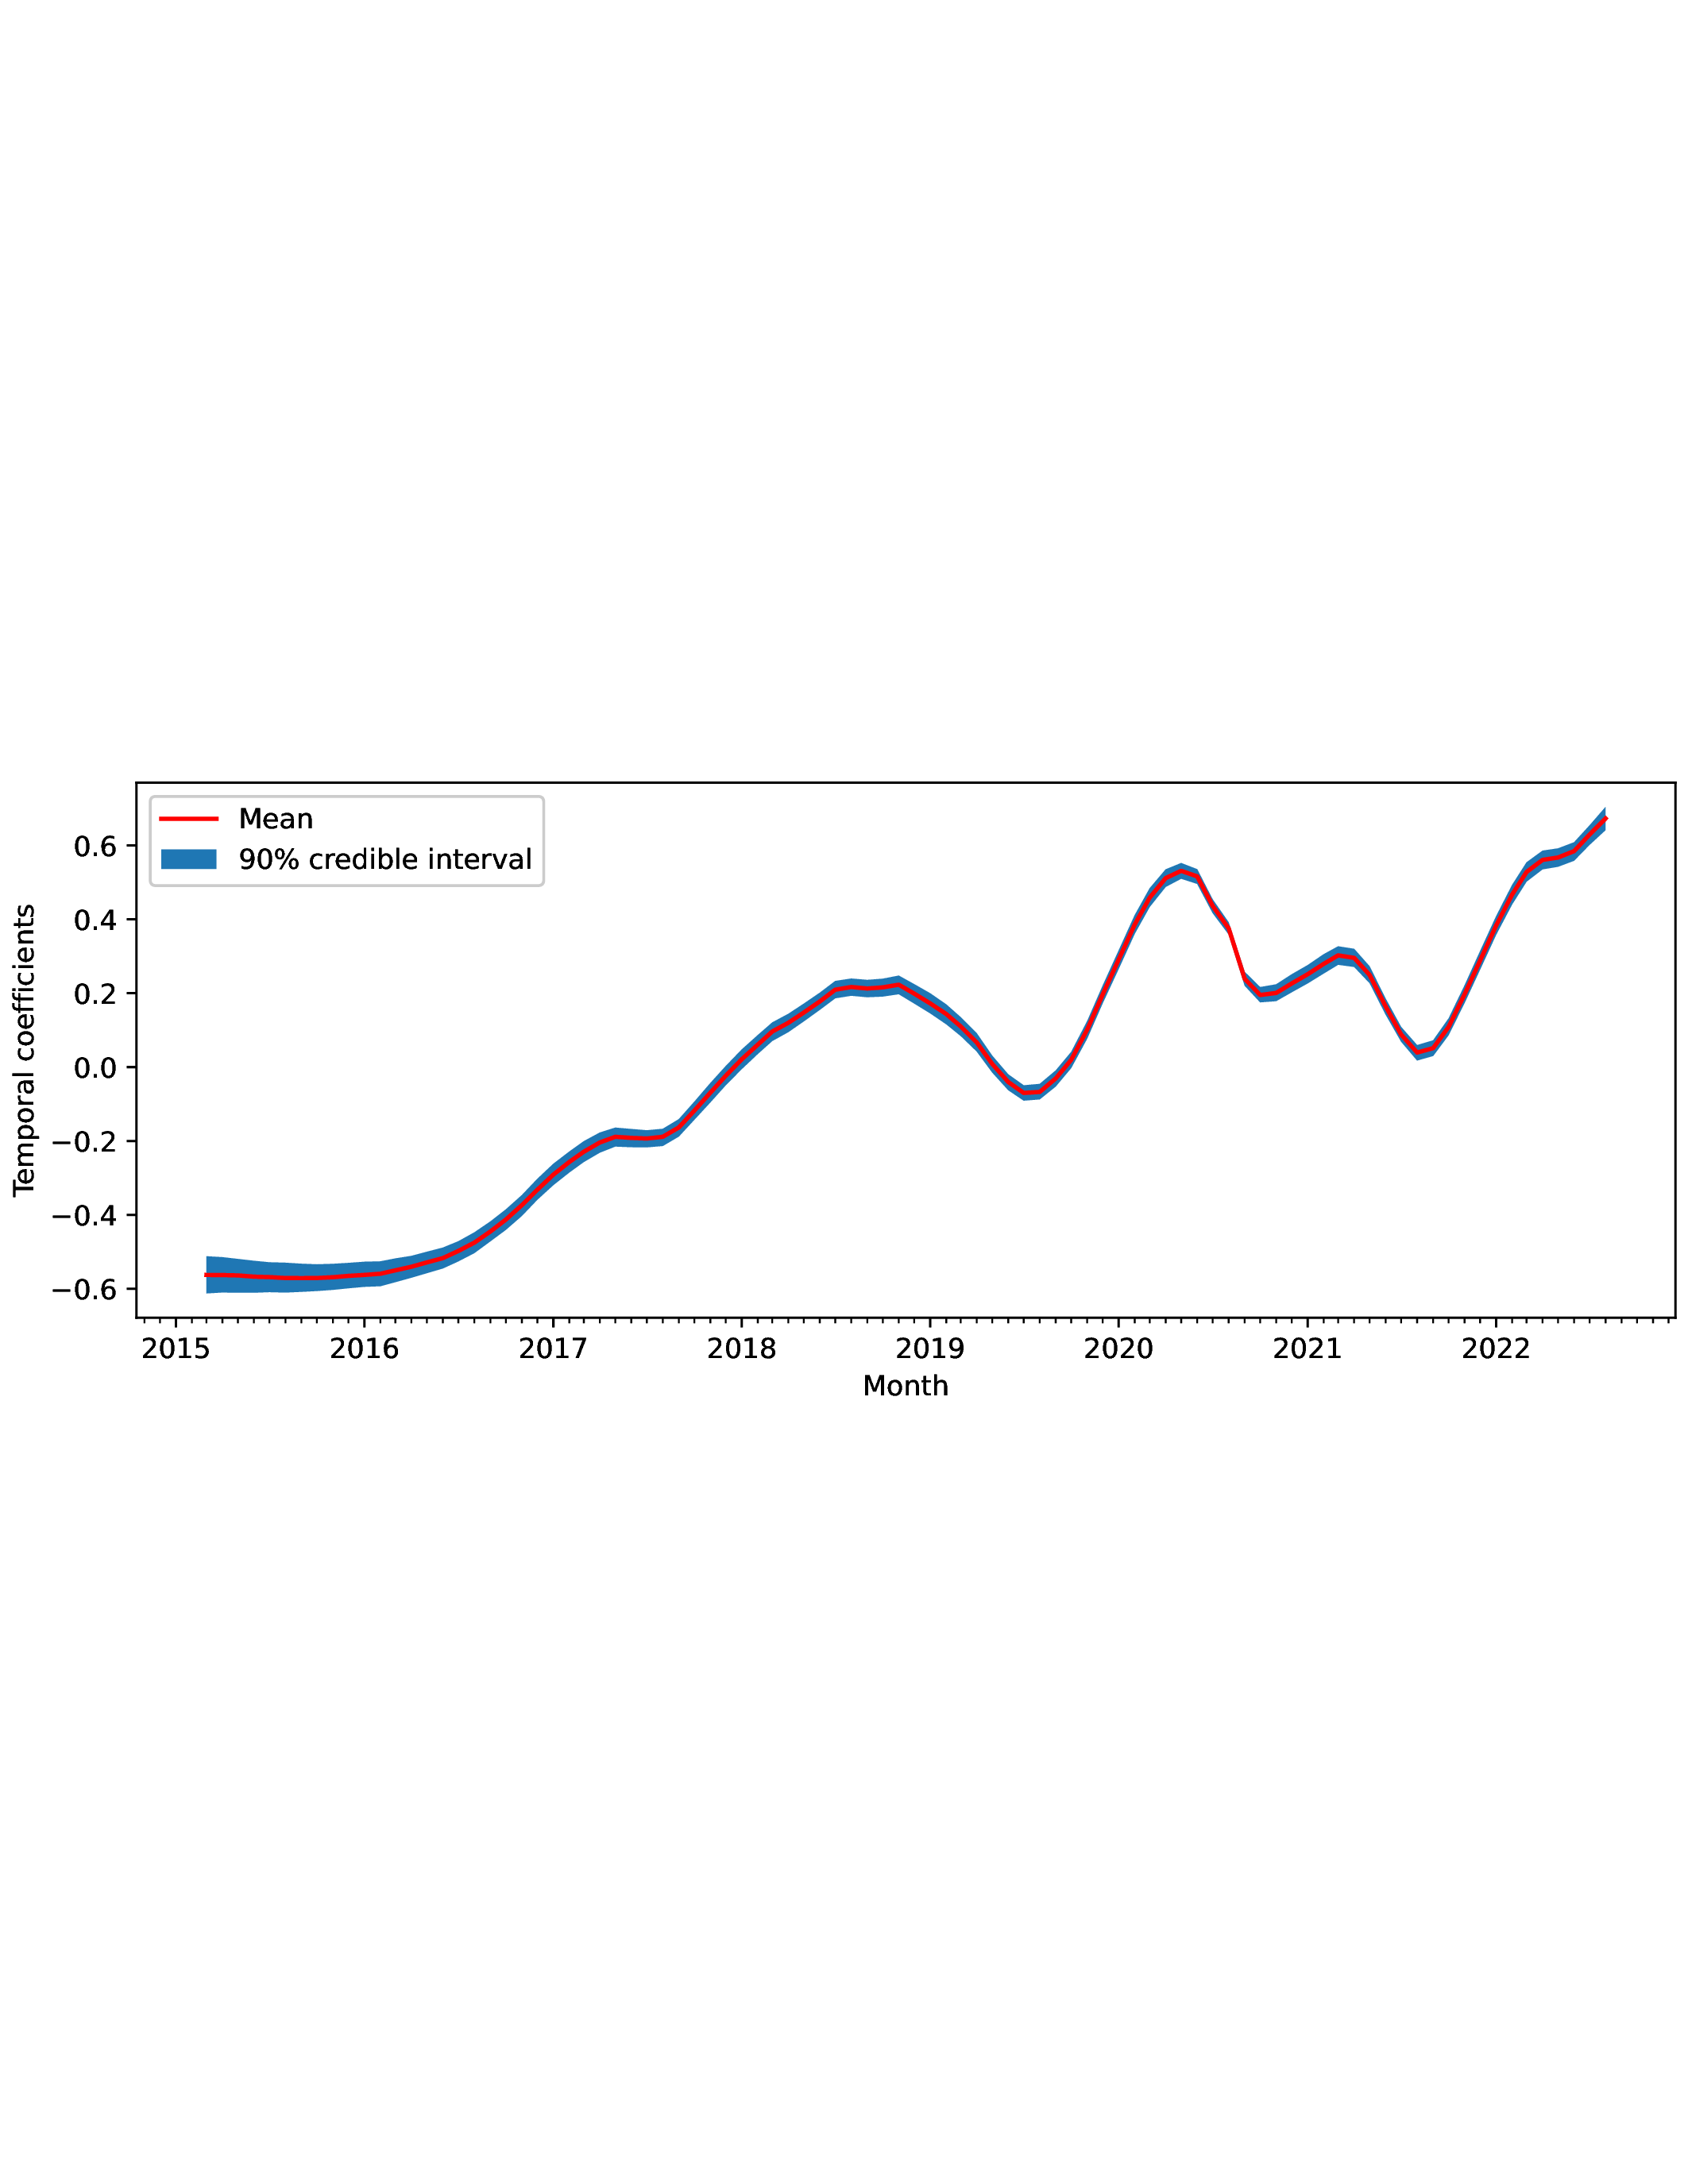}
	\caption{Coefficients for each monthly covariate in NYC, with 90\% credible intervals.}
	\label{fig:temporalcoefnyc}
\end{figure}

\begin{figure}[tb]
	\centering
	\includegraphics[width = .9\textwidth]{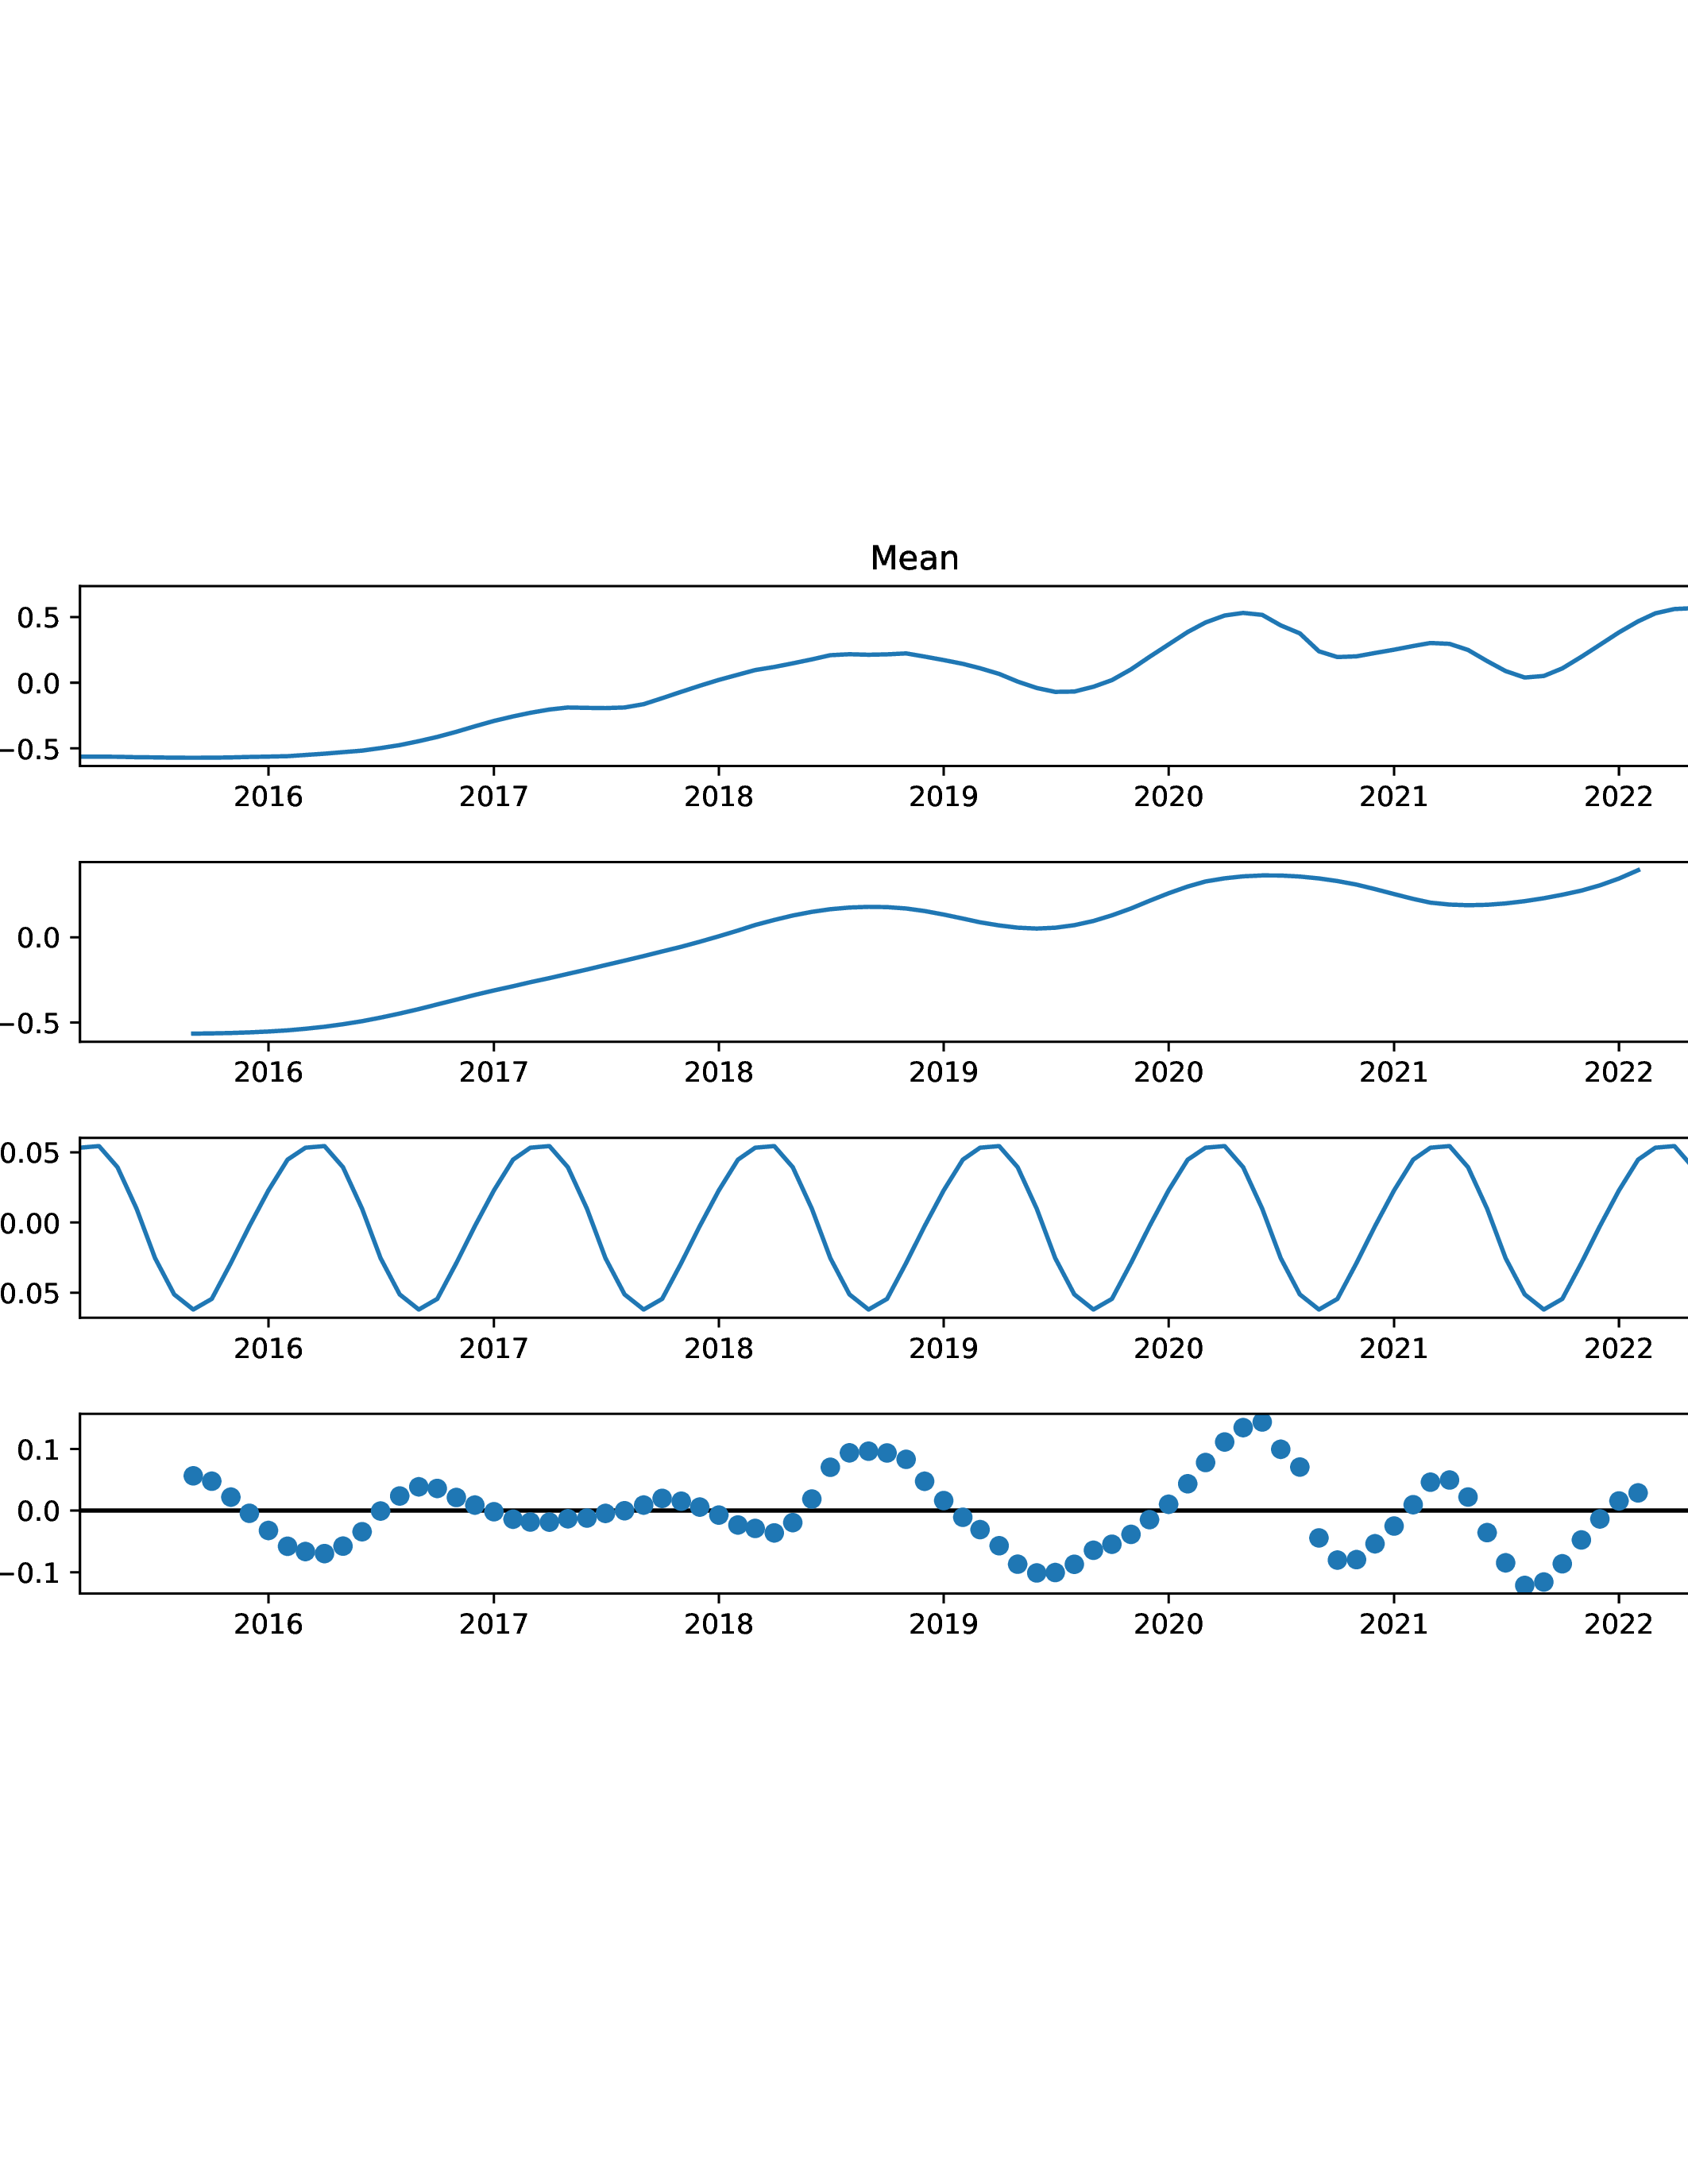}
	\caption{Seasonal decomposition of the mean of the coefficients for monthly covariates in NYC.}
	\label{fig:nyc_seasonal_decomp}
\end{figure}

\begin{figure}[tb]
	\centering
	\includegraphics[width = .8\textwidth]{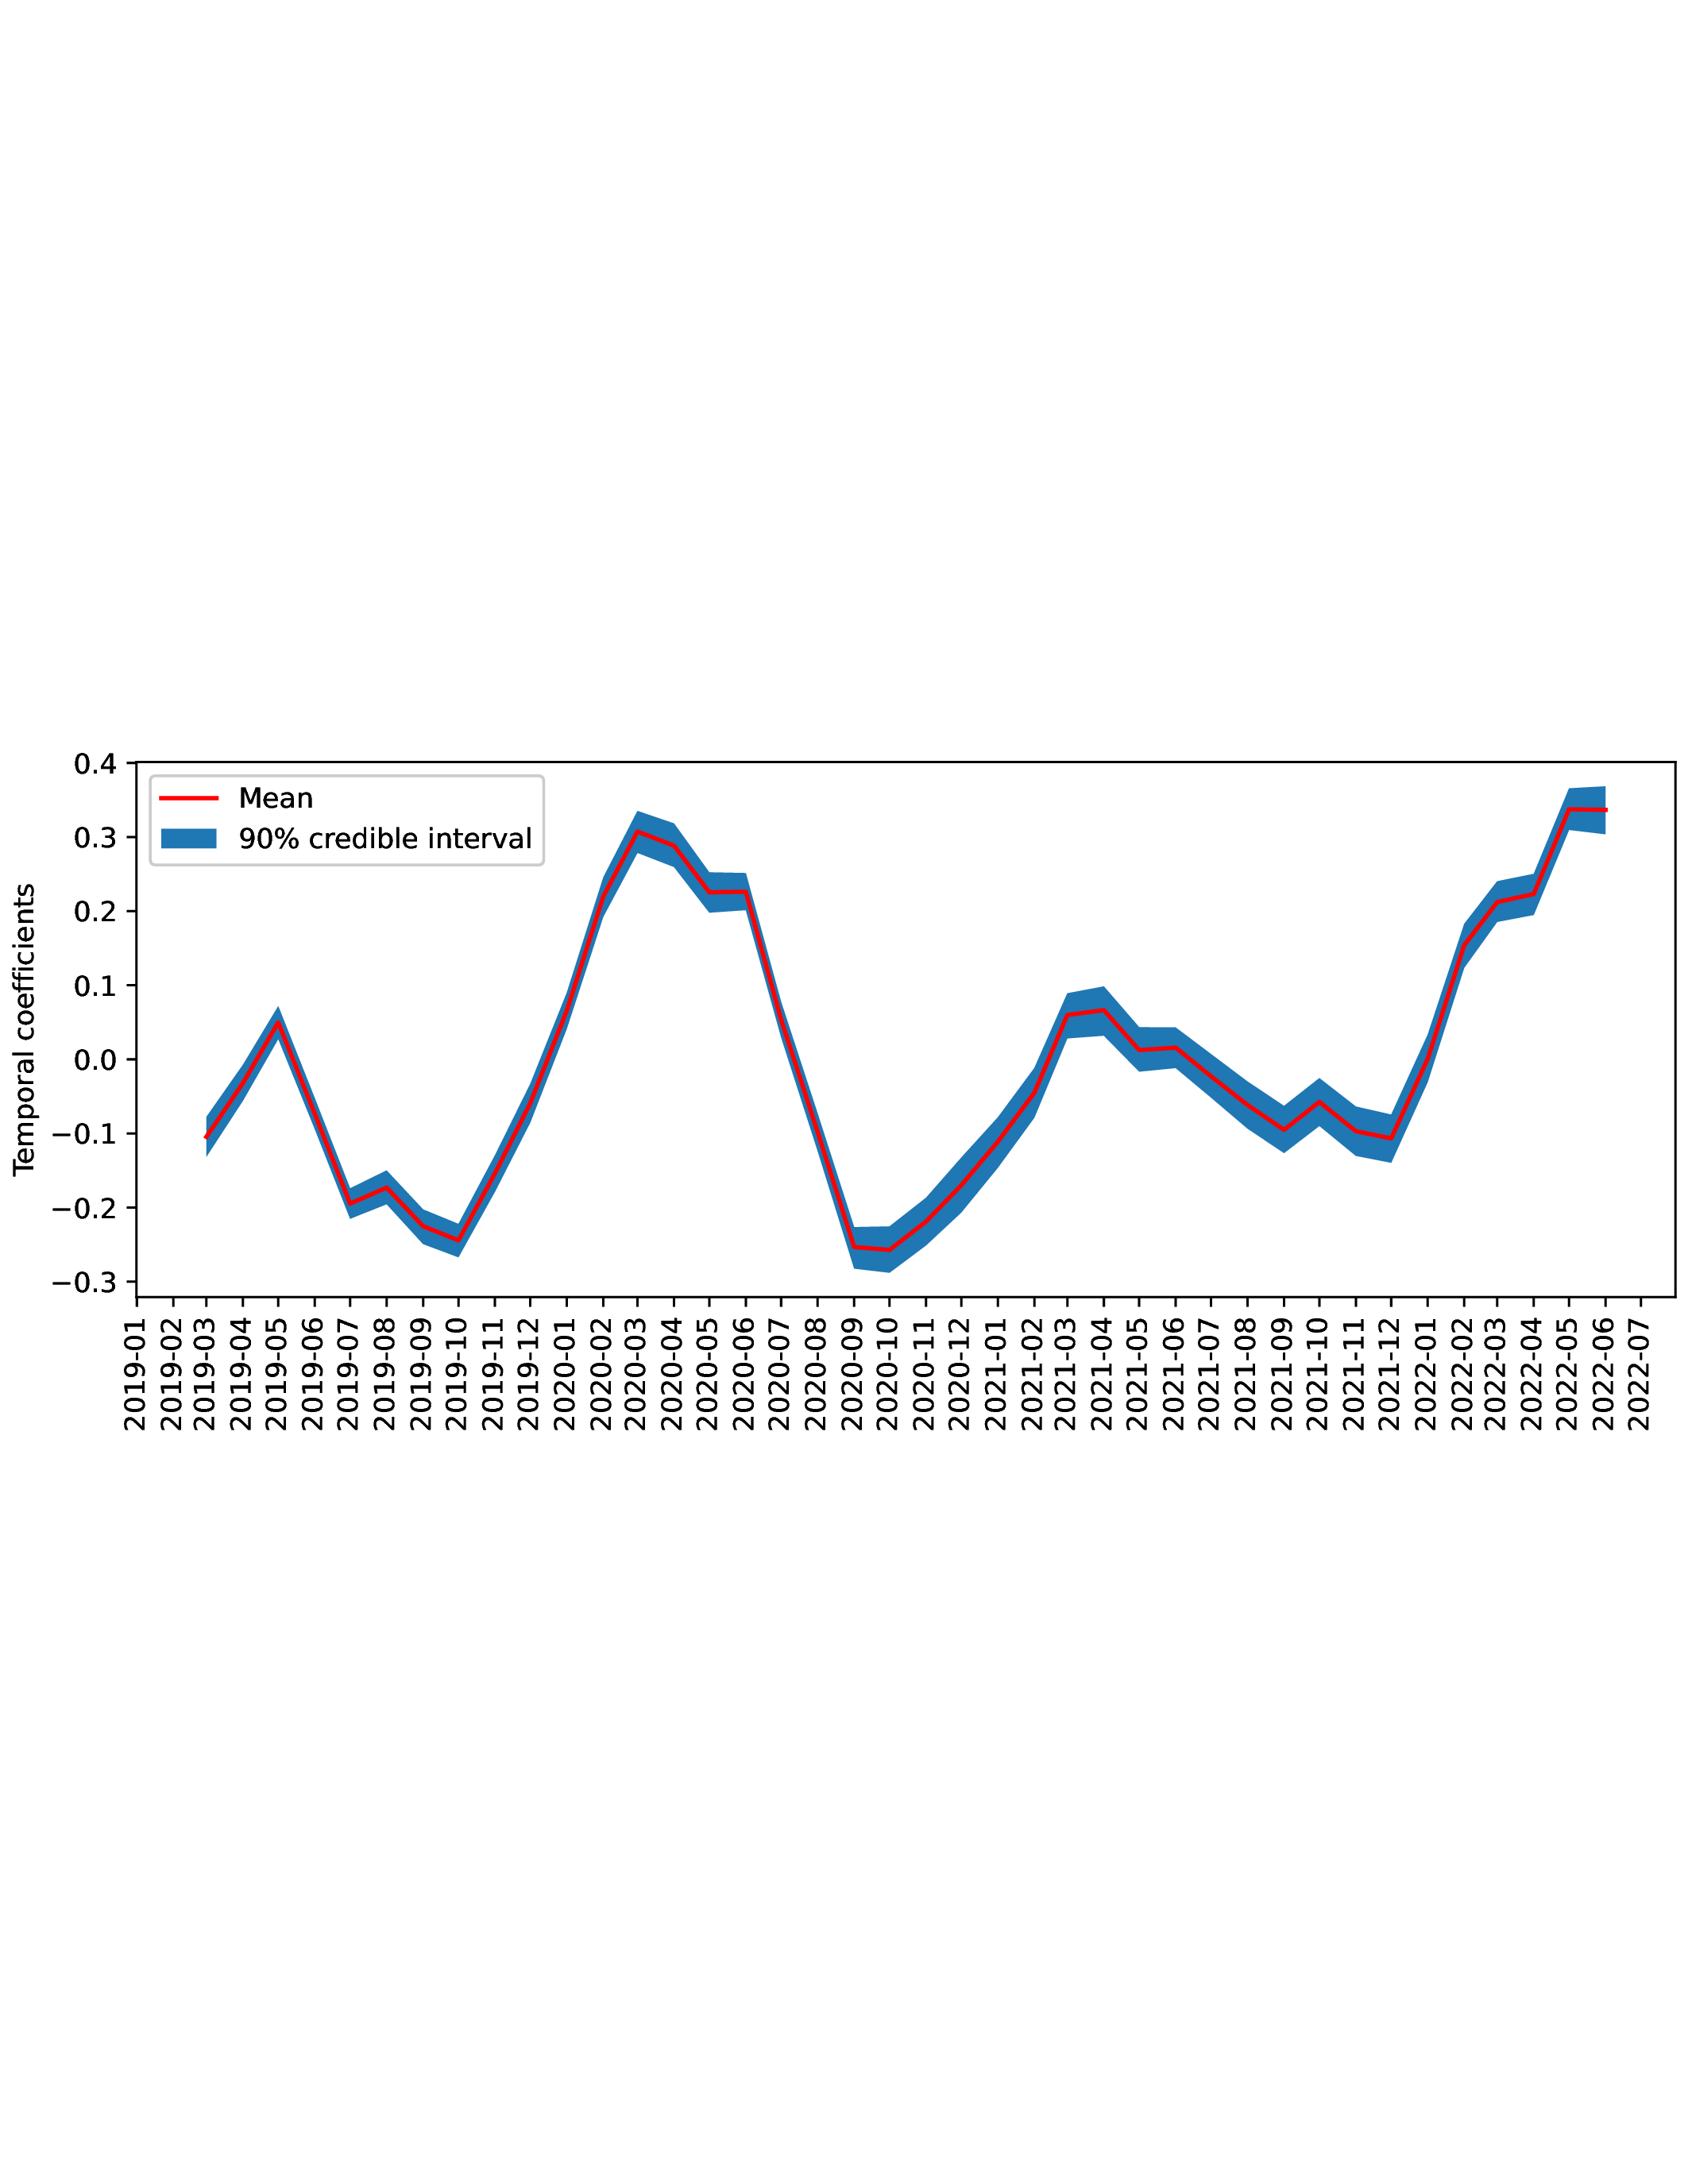}
	\caption{Coefficients for each monthly covariate in Chicago, with 90\% credible intervals.}
	\label{fig:temporalcoefchicago}
\end{figure}

\begin{figure}[tb]
	\centering
	\includegraphics[width = .9\textwidth]{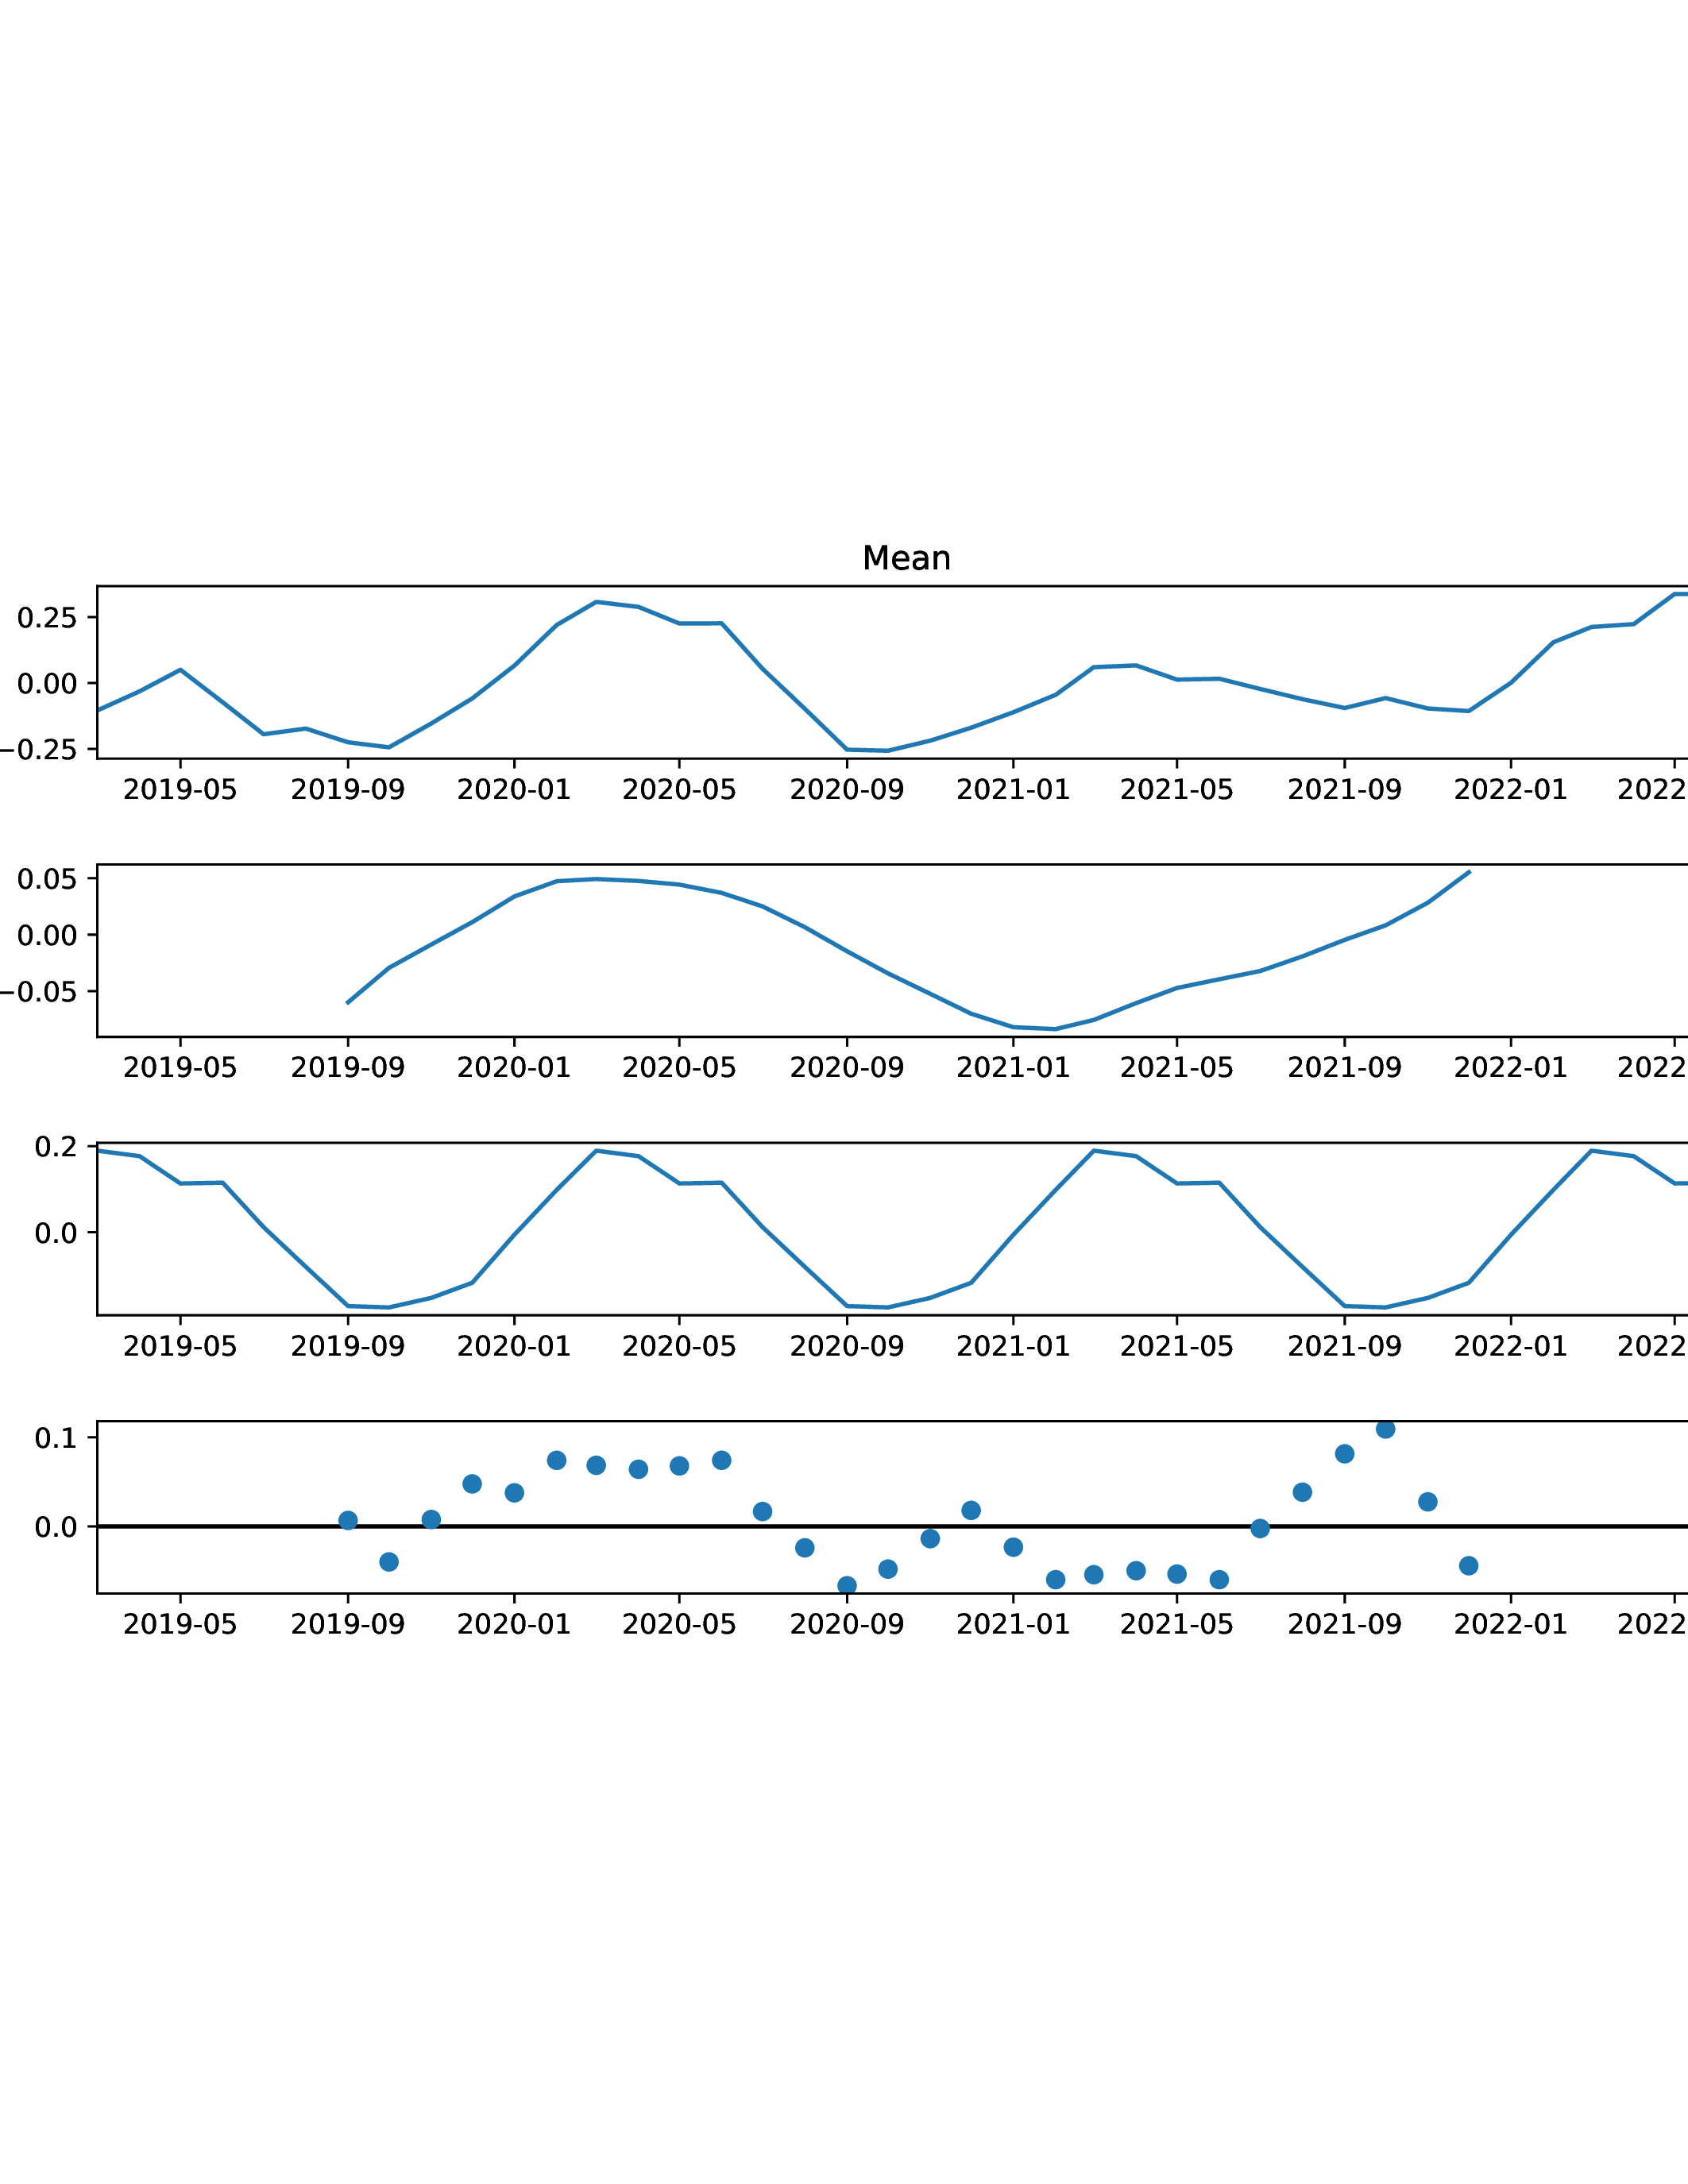}
	\caption{Seasonal decomposition of the mean of the coefficients for monthly covariates in Chicago. Compared with results from NYC, there is a significant amount of seasonal effect visible from the decomposition.}
	\label{fig:chicago_seasonal_decomp}
\end{figure}

\paragraph{Reporting seasonality} \Cref{fig:temporalcoefnyc} shows the mean and 90\% credible intervals of coefficients for each monthly covariate in NYC; treating the mean of these coefficients as a time series, \Cref{fig:nyc_seasonal_decomp} shows its decomposition. Reporting rates during the colder months (November through March) are higher while they are lower during the warmer months (April through October). This may be correlated with severe weather causing more serious incidents, but may also be associated with people's cautiousness during colder weather. Though the seasonal component may not seem substantial, it does represent a 1.5 times ($e^{0.4}$) difference in the seasonal effect alone; and when combined with the other effects, the monthly covariate large reporting rate variation over time. \Cref{fig:temporalcoefchicago} and \Cref{fig:chicago_seasonal_decomp} show similar results for Chicago data.

% \todo{maybe add more analysis?}
