# Supplementary material for: Quantifying Spatial Under-reporting Disparities in Resident Crowdsourcing
Source: arXiv:2204.08620 source file (2023-12-06)
Supplement: Supplementary file 2 [file appendix_proofs.tex]

\begin{figure}[tbh]
	\centering
	{
		\includegraphics[width=\textwidth]{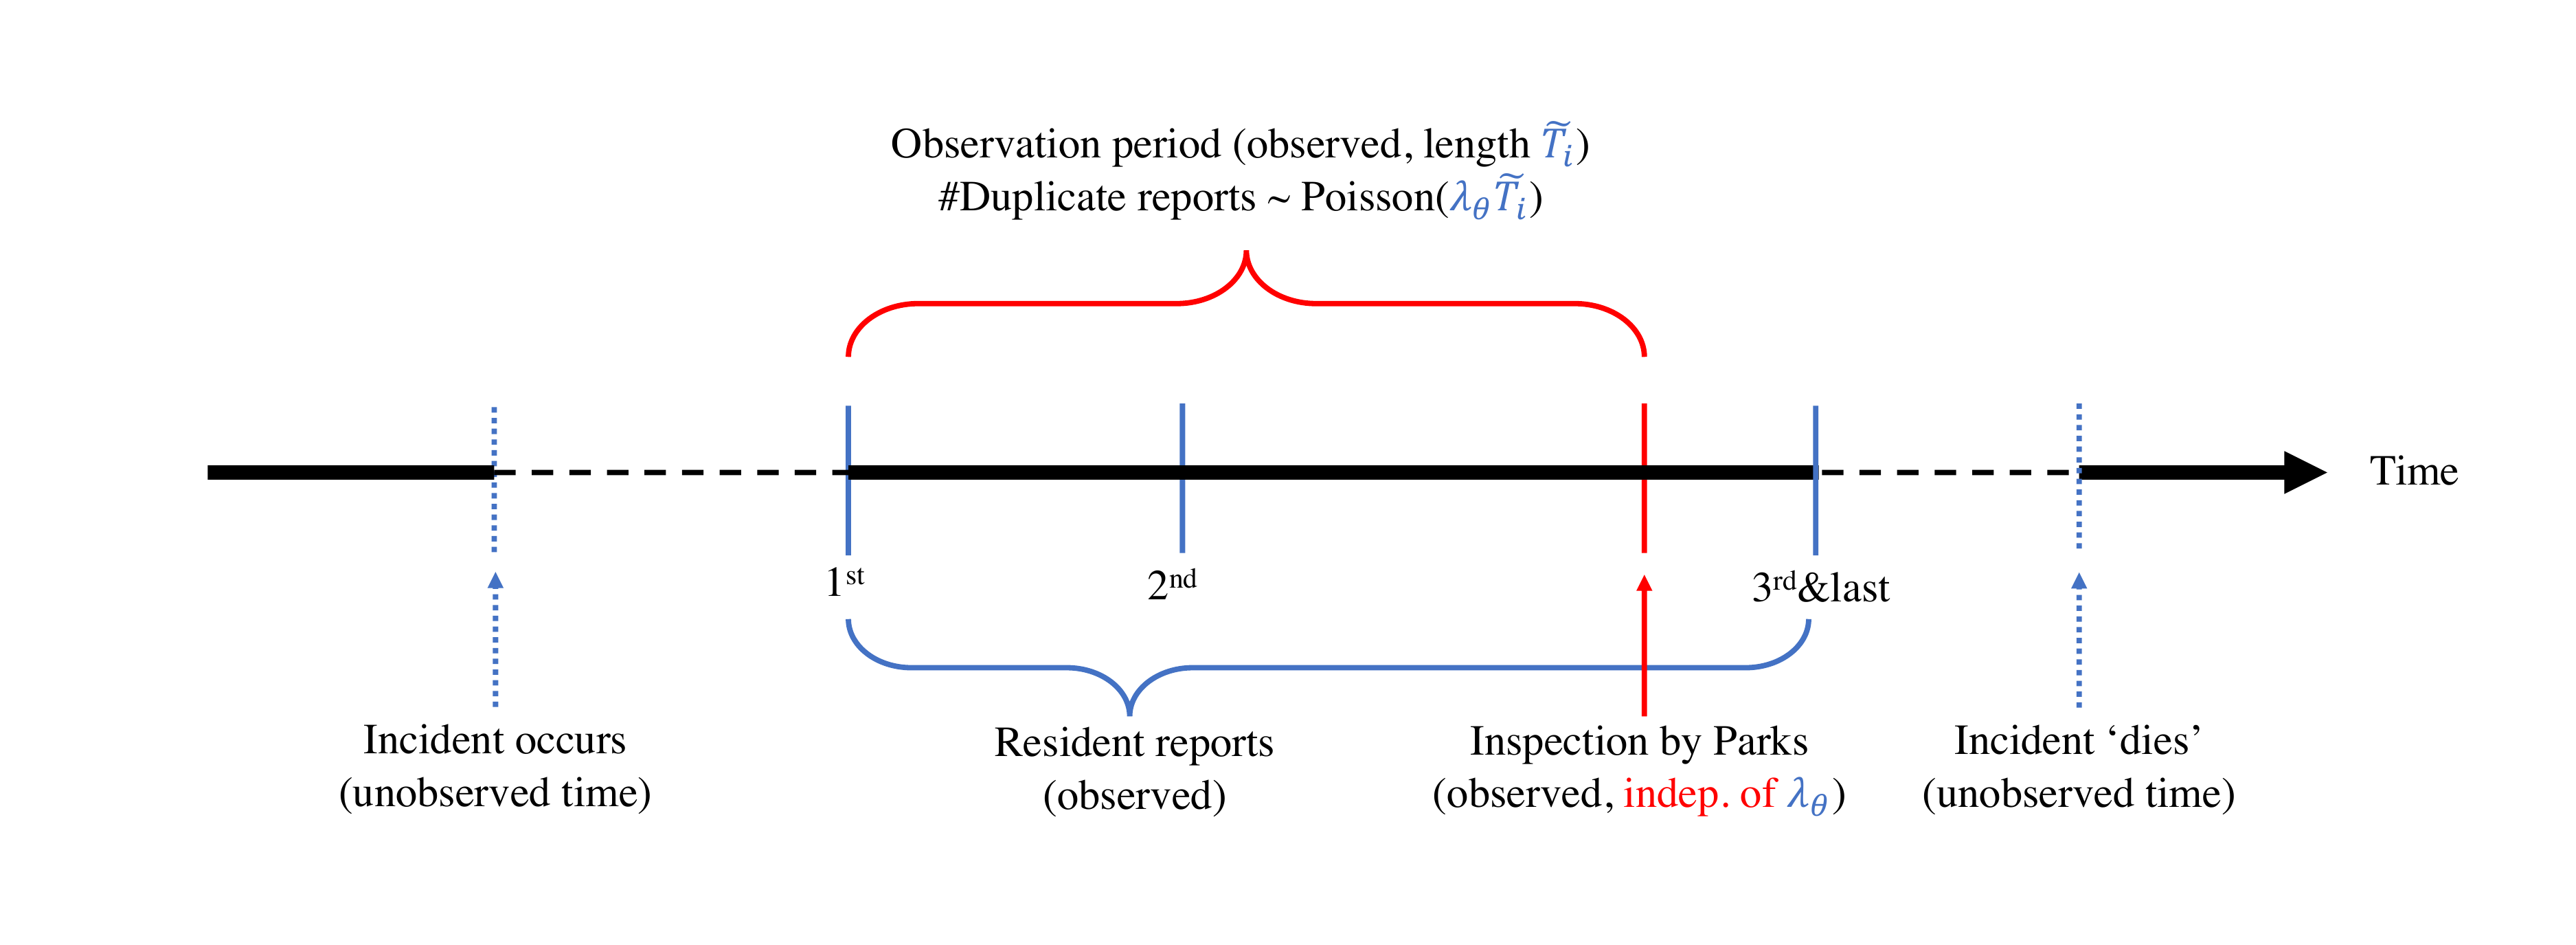}
		% 		\caption{Census tract fixed effects}
		% 		\end{subfigure}
	}
	\caption{Finding an observation period within which reports are Poisson. In \Cref{thm:stoppingtimes}, we establish a way to design an observation period, with both ends stopping times, independent of the reporting rate given the type. In the application, the start of this observation period is set to be the time of the first report, which is the first time we learn of this incident. The length of the observation period, $\tilde{T_i}$ is a design choice: in practice, we set the end of the observation period to be the earlier one of the inspection time and a time with fixed interval from the first report, thus satisfying the assumptions of being a stopping time and independence of reporting rate in \Cref{thm:stoppingtimes}. In this figure, we illustrate the case where the inspection time is the earlier of the two.}
			\label{fig:observation_gen}
\end{figure}

\propnonidenti*

\proof{Proof of Proposition \ref{prop:identi}.}

The proof of Proposition \ref{prop:identi} follows directly from the following Lemma.

\begin{lemma}\label{observed_rate}
Suppose each incident gets reported independently, and the distribution of the interval of reporting duration $T_i$ has density function $f(\cdot):[0,\infty)\mapsto \mathbb{R}$. Then under steady state, $N_\theta^{\obs}$ follows a Poisson process with rate $\Lambda_{\theta}'$, where
$$
\Lambda_{\theta}' = \Lambda_{\theta}\left[1-\int_{0}^\infty\exp\left(-\int_{0}^t\lambda_{\theta}(u)du\right)f(t)dt\right].
$$

In the simplest time homogenous case, this rate simplifies to:
$$
\Lambda_{\theta}' = \Lambda_{\theta}\left[1-\int_{0}^\infty\exp\left(-\lambda_\theta t\right)f(t)dt\right].
$$
\end{lemma}

\proof{Proof.}
Let $m(t)$ be the number of times an incident is reported in an interval of $t$, starting from its birth. We know from the model assumption that $m(t)$ follows a Poisson distribution:
$$
m(t)\sim \text{Poisson}\left(\int_0^t\lambda_\theta(u)du\right).
$$

Under steady state, each unique incident gets reported with probability
\begin{align*}
p &= \int_{0}^{\infty}\text{Pr}[m(t)\ge 1|T_i=t]f(t)dt\\
&=\int_{0}^\infty \left[1-\exp\left(-\int_{0}^t\lambda_{\theta}(u)du\right)\right]f(t)dt\\
&= 1-\int_{0}^\infty\exp\left(-\int_{0}^t\lambda_{\theta}(u)du\right)f(t)dt,
\end{align*}
which simplifies under time-homogeneity to
\begin{align*}
p &= 1-\int_{0}^\infty\exp\left(-\lambda_{\theta}t\right)f(t)dt.
\end{align*}

Over a time interval of $t$, the total number of incidents of type $\theta$ that happen, $N_\theta(t)$ follows a Poisson process with rate $\Lambda_\theta$. Conditional on $N_\theta(t)=n, n=0,1,\dots$, under steady state, $N_{\theta}^\obs(t)$ follows a binomial distribution with parameters $(n,p)$. Thus $N_{\theta}^\obs(t)$ follows a Poisson distribution with rate $\Lambda_\theta p$, which completes the proof.\Halmos

\endproof

Lemma \ref{observed_rate} establishes that the rate at which we observe unique incidents depends on a lot of various aspects. Under steady state, $N_{\theta}^\obs$ follows a Poisson process with parameter $\Lambda_\theta'$, where $\Lambda_\theta'$ is a function of the incident happening rate $\Lambda_\theta$ the (potentially non-homogenous) reporting rate $\lambda_\theta(\cdot)$ and the distribution of reporting duration $f(\cdot)$.

% To restate Lemma \ref{observed_rate}, we have that under steady state,
% $$
%  \frac{N_\theta^\obs(T)}{T} \sim \text{Poisson}\left(\Lambda_{\theta}'\right),
% $$
% where
% $$
% \Lambda_{\theta}' = \Lambda_{\theta}\left[1-\int_{0}^\infty\exp\left(-\lambda_\theta t\right)f_{T}(t)dt\right].
% $$

In practice, when the observation period length $T$ is large, we can safely assume that for each period $[\tau,\tau+1), \tau=0,\dots,T$, the observed reports  $N_\theta^\obs\left([\tau,\tau+1]\right)$ are close to steady state, and thus follow independent and identical Poisson$(\Lambda_\theta')$ distribution. Following the law of large numbers we get
$$
\lim_{T \to \infty} \frac{N_\theta^\obs(T)}{T} = \lim_{T \to \infty} \frac{\sum_{\tau=0}^{T-1}N_\theta^\obs\left([\tau,\tau+1]\right)}{T} = \mathbb{E}\left[N_\theta^\obs\left(1\right)\right]=\Lambda_{\theta}'.
$$

Thus, if we are only using information about the unique incidents, it is impossible to determine $\lambda_\theta$ without having full knowledge about both $\Lambda_\theta$ and $f(\cdot)$.
\Halmos %However, in reality, the latter two quantities are extremely difficult to estimate, this stems from the fact that all we can observe is a biased and noisy sample, which is particularly true for the distribution of reporting time $f(\cdot)$. This argument leads to the validity of Proposition \ref{prop:identi}.

\endproof

\thmst*

\proof{Proof of Theorem \ref{thm:stoppingtimes}.}
The result immediately follows for $ \tilde T_i$ independent of the sample path (i.e., a constant $\tilde T_i$), from standard Poisson results.

We prove the result for each possible set of inter-arrival times for reports; let $t_i^m$ for $m  \in \{1, \dots \tilde M_i + 1\}$ be the inter-arrival time between the $(m-1)$th and $m$th reports, with $t_i^{m}$ for $m=0$ defined as  the time between the interval start and the first report, and for $m=\tilde M_i+1$ defined as  the time between the last report and interval end. Thus, we have $\sum_{m=1}^{\tilde M_i+1} t_i^m = \tilde T_i$.

%We observe $\{t_i^m\}_{m = 1}^{\tilde M_i+1}$.
%, where $m=0$ corresponds to time between incident birth and first report, and
%but not $t_i^0$, the time between incident birth the first report, as we do not observe the incident birth time $t_i$.
%Thus, we have $\tilde t_i = t_i^0 + t_i$, and $\sum_{m=1}^{\tilde M_i} t_i^m = \tilde T_i$.

We prove that $\tilde{Pr}({D_i, \{t_i^m\}} | \lambda(\cdot)) = {Pr}({D_i}, \{t_i^m\} | \lambda(\cdot)) g({D_i}, \{t_i^m\})$ for each valid $\{t_i^m\}$ and $i$, and so the first part of the result follows. The proof follows from writing down the likelihood function of the interrarival times and data, and noticing that the stopping times likelihoods decompose in way that they just depend on the sample path, and not $\lambda (\cdot)$.

% \todo{probably some more text here about sample paths, etc.}

~\\\noindent $\tilde{Pr}({D_i, \{t_i^m\}} | \lambda(\cdot)) $
\begin{align*}
= &\prod_{m=1}^{\tilde M_i}\left[\bbP\left(\text{interrarival } t_i^m\text{, and } \tilde T_i >  \sum_{j=1}^{m} t_j^m | \lambda, m, \{t_i^j\}_{j=1}^m\right)\right] \bbP\left(\text{die before the }(\tilde M_i+1)\text{th report} | \lambda, \tilde M_i, \{t_i^j\}_{j=1}^{\tilde M_i} \right)\\
= &\prod_{m=1}^{\tilde M_i}\left[\bbP\left(t_i^m | \lambda, m, \{t_i^j\}_{j=1}^m\right) \bbP\left(\tilde T_i >  \sum_{j=1}^{m} t_j^m | \lambda, m, \{t_i^j\}_{j=1}^m\right)\right] \\
&\times \bbP\left(\text{interrarival} >  t_i^{\tilde M_i+1} | \lambda, \tilde M_i, \{t_i^j\}_{j=1}^{\tilde M_i} \right) \bbP\left(\text{death time is } t_i^{\tilde M_i+1} | \lambda, \tilde M_i, \{t_i^j\}_{j=1}^{\tilde M_i}\right)\\
= &\left[\prod_{m=1}^{\tilde M_i}\left[\bbP\left(t_i^m | \lambda, m, \{t_i^j\}_{j=1}^m\right)\right]\bbP\left(\text{interrarival} >  t_i^{\tilde M_i+1} | \lambda, \tilde M_i, \{t_i^j\}_{j=1}^{\tilde M_i} \right)\right]\\
&\times\left[\prod_{m=1}^{\tilde M_i}\left[\bbP\left(\tilde T_i >  \sum_{j=1}^{m} t_j^m | \lambda, m, \{t_i^j\}_{j=1}^m\right)\right]\bbP\left(\text{death time is } t_i^{\tilde M_i+1} | \lambda, \tilde M_i, \{t_i^j\}_{j=1}^{\tilde M_i}\right)\right]
 \\
\intertext{By assumption, $\tilde T_i$ is a stopping time, and independent of $\lambda$ given the history. Thus, we can drop the conditioning on $\lambda$ on the second half of the equation.}
= &\left[\prod_{m=1}^{\tilde M_i}\left[\bbP\left(t_i^m | \lambda, m, \{t_i^j\}_{j=1}^m\right)\right]\bbP\left(\text{interrarival} >  t_i^{\tilde M_i+1} | \lambda, \tilde M_i, \{t_i^j\}_{j=1}^{\tilde M_i} \right)\right]\\
&\times\left[\prod_{m=1}^{\tilde M_i}\left[\bbP\left(\tilde T_i >  \sum_{j=1}^{m} t_j^m | m,\{t_i^j\}_{j=1}^m\right)\right]\bbP\left(\text{death time is } t_i^{\tilde M_i+1} | M_i, \{t_i^j\}_{j=1}^{\tilde M_i}\right)\right] \\
= &\left[\prod_{m=1}^{\tilde M_i}\left[\bbP\left(t_i^m | \lambda, m, \{t_i^j\}_{j=1}^m\right)\right]\bbP\left(\text{interrarival} >  t_i^{\tilde M_i+1} | \lambda, \tilde M_i, \{t_i^j\}_{j=1}^{\tilde M_i} \right)\right] g(D_i, \{t_i^m\})
\end{align*}%

The first part of the result follows by marginalizing out $\{t_i^m\}$, as the term inside the first square bracket is exactly the likelihood of inter-arrival times for a (potentially non-homogeneous) Poisson distribution. Note that the decomposition does not hold without each value being a stopping time.

In the homogeneous case, we have
\begin{align*}
\tilde{Pr}({D_i, \{t_i^m\}} | \lambda(\cdot)) &= \left[\prod_{m=1}^{\tilde M_i}\left(\lambda \exp(-\lambda t_i^m)\right)\exp(-\lambda t_i^{\tilde M_i + 1})\right]g(D_i, \{t_i^m\}) \\
\intertext{Combining this for multiple incidents, we get the log-likelihood function for the reporting rate $\lambda$:}
\log L(\lambda) &= \sum_{i}\left[\sum_{m=1}^{\tilde M_i}\left[\log \lambda - \lambda t_i^{m} \right] - \lambda t_i^{\tilde {M}_i + 1} + \log g(D_i, \{t_i^m\}) \right],\\
\intertext{by the first order condition $\frac{d}{d\lambda} \log L(\lambda) = 0$ we get:}
\sum_{i}\left[\sum_{m=1}^{\tilde M_i}\left[\frac{1}{\lambda} - t_i^m \right] - t_i^{\tilde M_i + 1}\right] = 0 &\Rightarrow \hat{\lambda}^{MLE} = \frac{\sum_i {\tilde M_i}}{\sum_i \sum_{m=1}^{\tilde M_i + 1} t_i^m} = \frac{\sum_i {\tilde M_i}}{\sum_i \tilde T_i} \Halmos%= \frac{\sum_i {M_i-1}}{\sum_i  (T_i-t_i)}.
\end{align*}
\endproof
