# Supplementary material for: Quantifying Spatial Under-reporting Disparities in Resident Crowdsourcing
Source: arXiv:2204.08620 source file (2023-12-06)
Supplement: Supplementary file 4 [file appendix_analysis.tex]

\subsection{Additional information}

% \todo{add 1 sentence referencing each table/figure and what it includes}

In this section, we provide some additional information about our dataset and results. \Cref{tab:desc} provides description of the covariates selected; \Cref{fig:reginccoef} shows the relationship between number of unique incidents observed versus the census tract fixed effect; \Cref{fig:posteriors} shows the posterior distribution of number of reports as estimated by the basic Poisson regression model, and the zero inflated Poisson regression model, with reference to the observed distribution; \Cref{tab:coeffull} lists the full information of the coefficients for census tract demographic covariates as estimated alone in a regression alongside the incident-specific covariates and the borough fixed effects.

% \begin{figure}[tb]
%	\centering
%	\begin{subfigure}[b]{0.42\textwidth}
%		\centering
%		\includegraphics[width=\textwidth]{plots/tract_hierarchy_zeroinflated_hiertract11medpriornocens2_dur100_repmedium_300300-1nocens2_censusmap}
%		\caption{Census tract fixed effects}
%		\label{fig:spatialmap}
%	\end{subfigure}
%	\hfill
%	% 	\begin{subfigure}[b]{0.56\textwidth}
%	% 		\centering
%	% 		\includegraphics[width=\textwidth]{plots/prop_states_box}
%	% 		\caption{Partisan lean distribution under STV and PAV}
%	% 		\label{fig:propbystatebox}
%	% 	\end{subfigure}
%	\caption{}
%	\label{fig:spatialheterog}
%\end{figure}

\input{plots/tab_covariates}

 \begin{figure}[tb]
	\centering
	\subfloat[][Reported incidents vs trees]{
		\includegraphics[width=.45\textwidth]{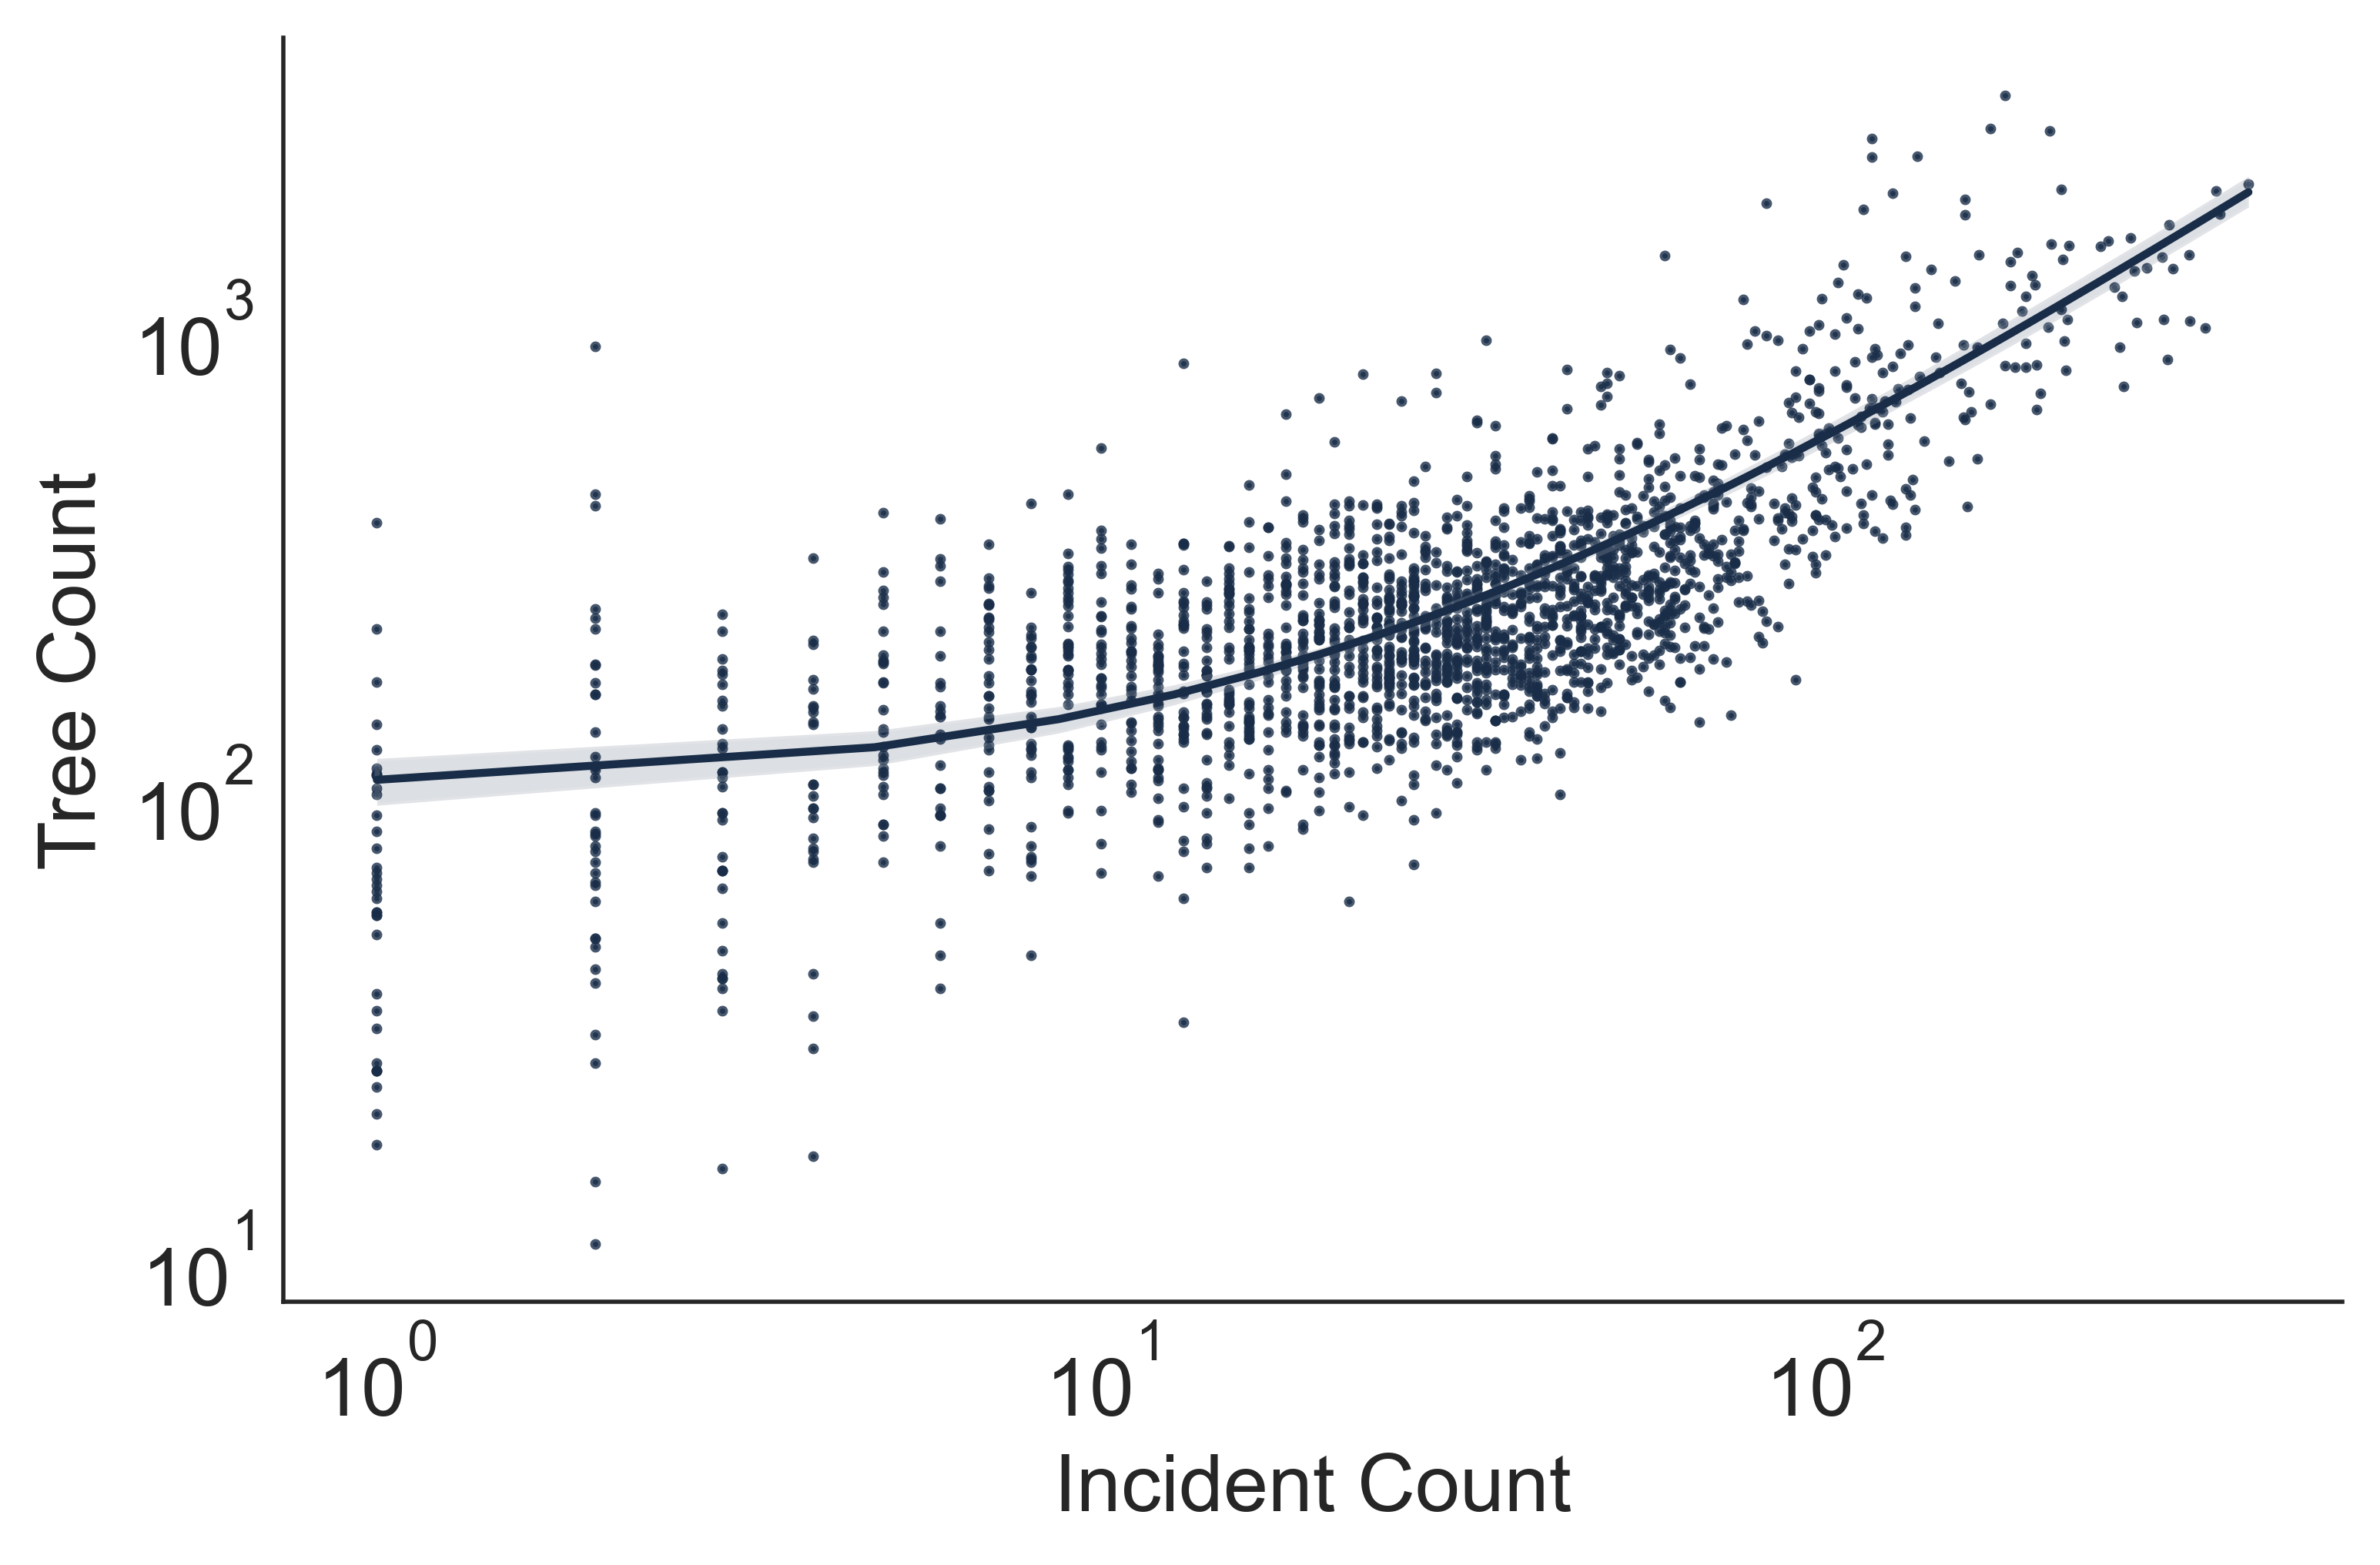}
		\label{fig:treesincidents}
	}
	\hfill
	\subfloat[][Incidents/Tree vs Census Tract Coefficient]{
	\includegraphics[width=.45\textwidth]{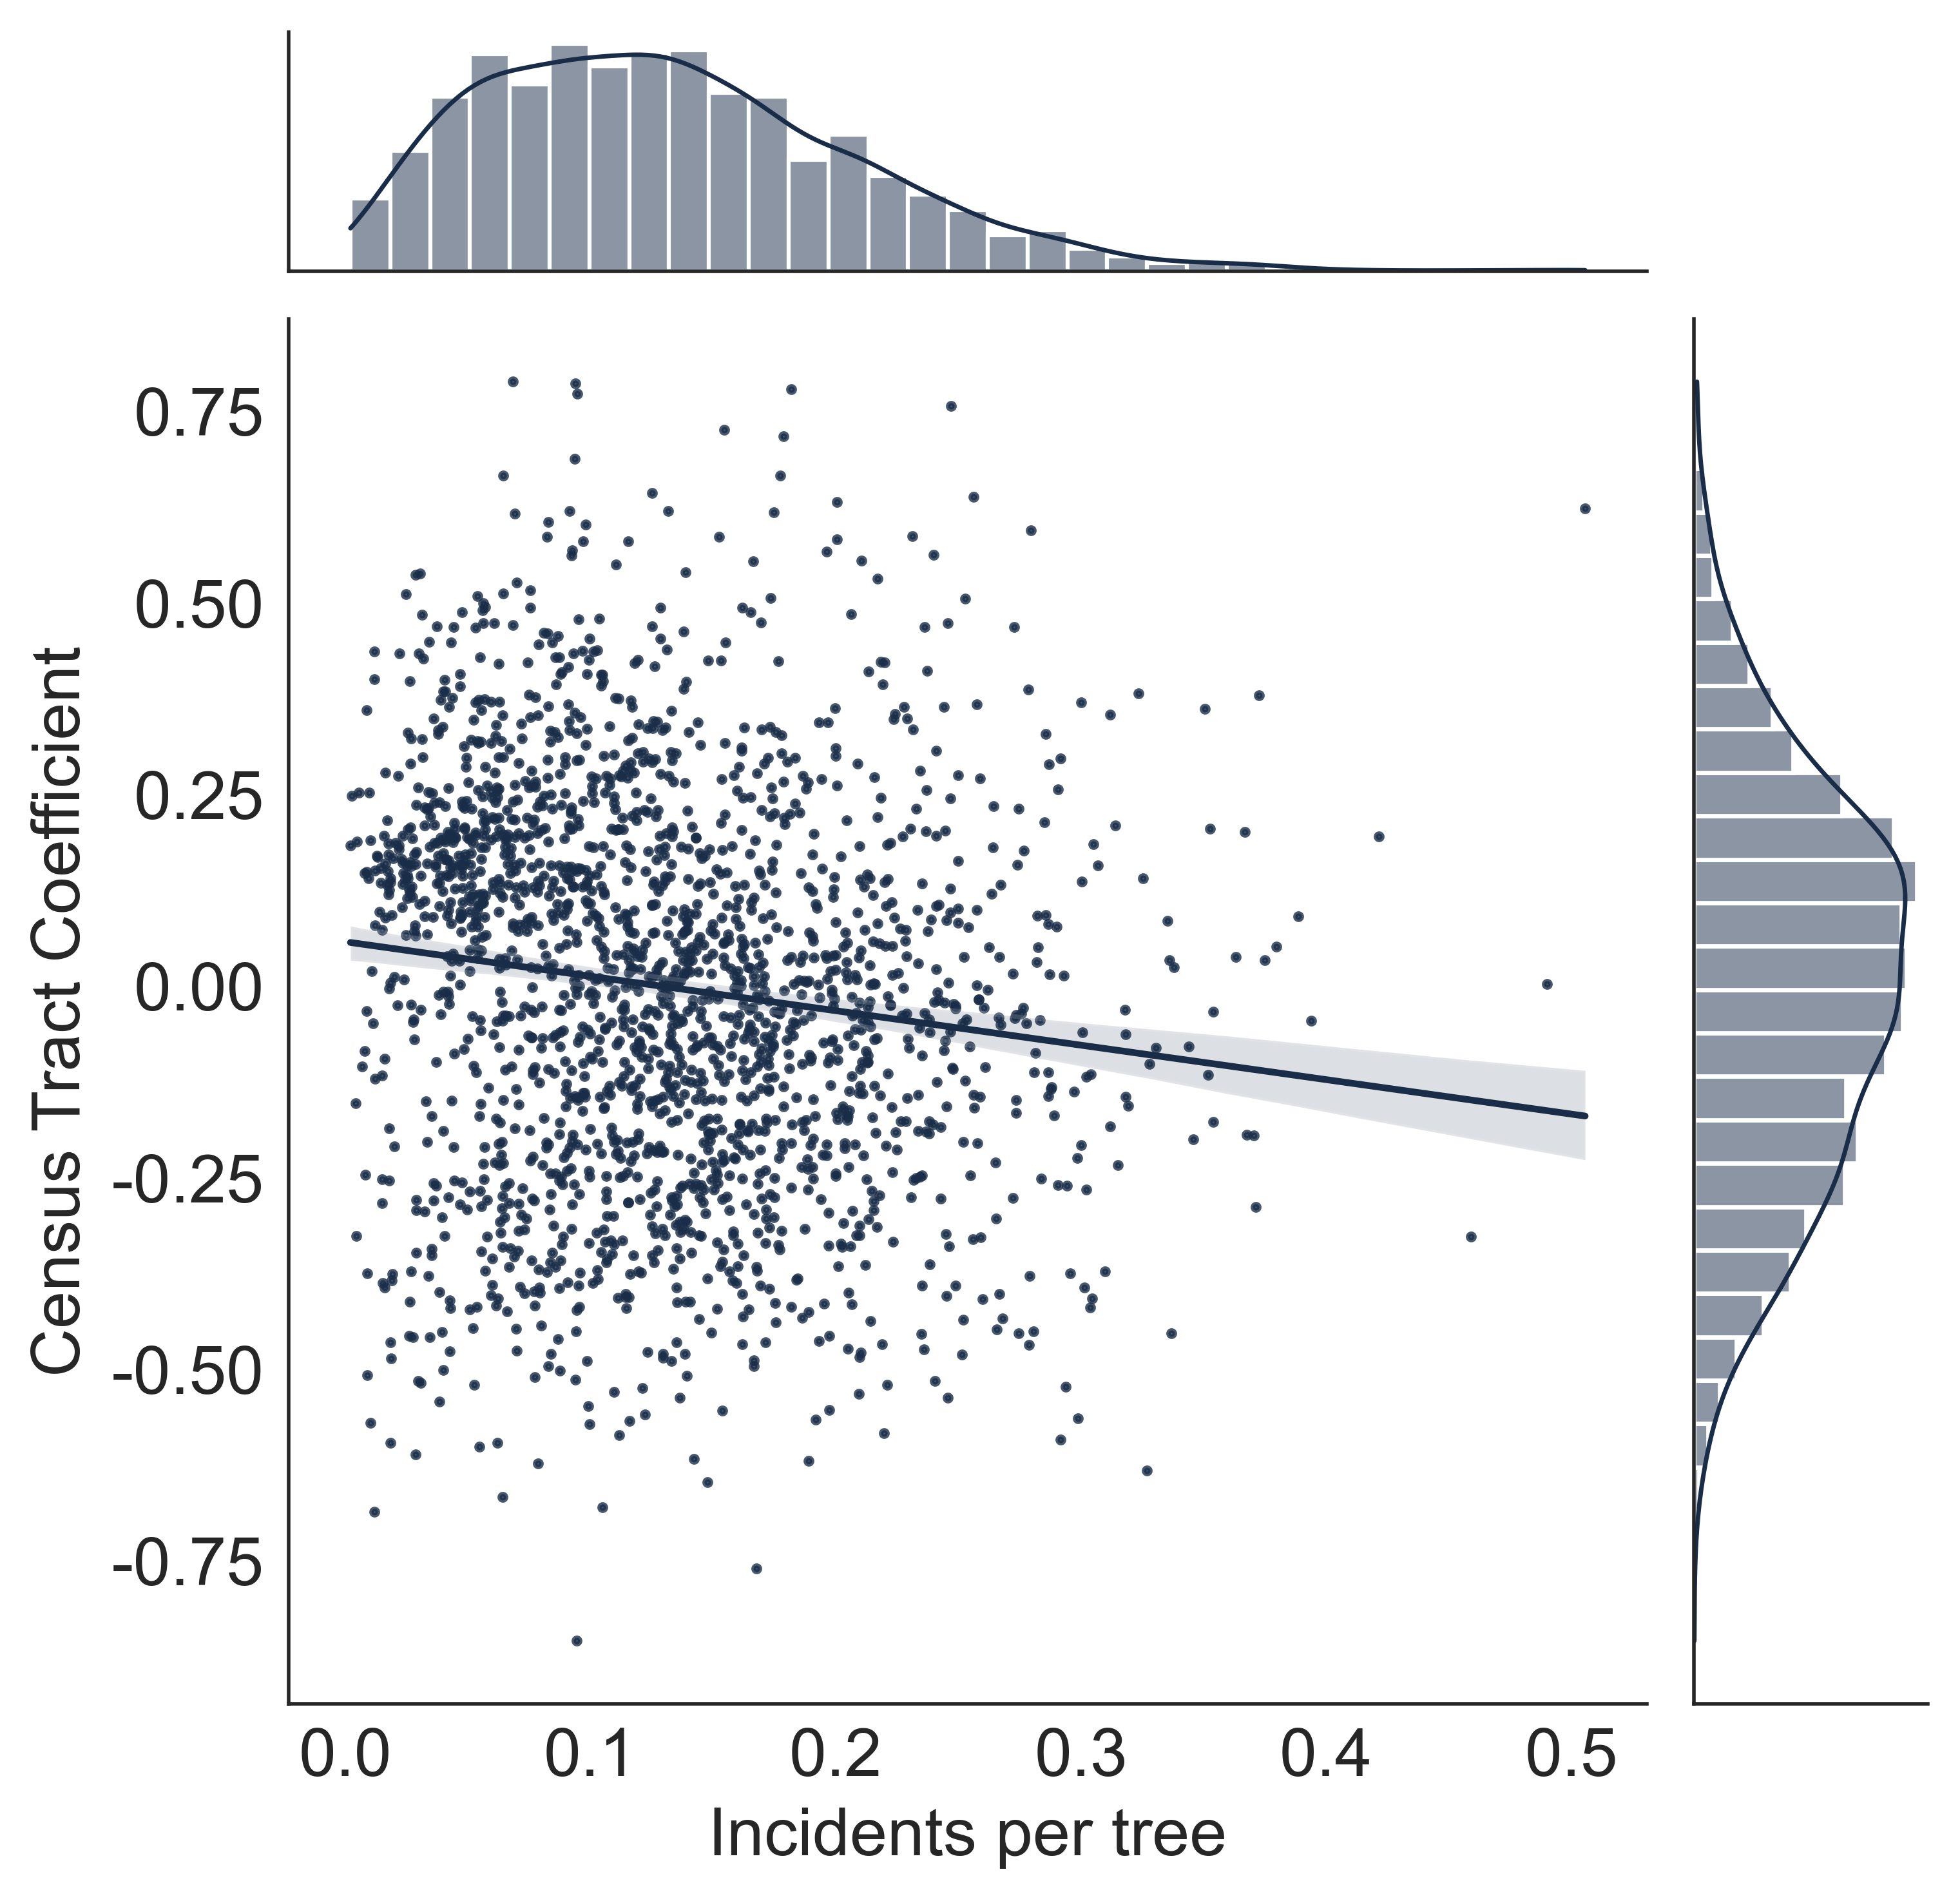}
	\label{fig:reginccoef}
}
	\caption{(a) For each census tract, the number of trees according to the 2015 New York Street Tree Census versus the number of reported incidents in that census tract. As expected, more trees results in more reported incidents. (b) 	The relationship between reported incidents per tree and the census tract fixed effect. The value, ``incidents per tree'' is an attempt to normalize the number of incidents we observe with the number we expect to observe -- and thus the ratio is a measure of \textit{reporting} rates as is done in prior work. We observe a slight negative relationship with this measure and the one we develop, the census tract coefficient in the Poisson regression. While it is possible that one can construct better proxies for how many incidents we expect to observe than the raw counts of trees, the relationship suggests that our method's results can differ substantially from those of prior work. We prefer our measure, as it automatically controls for `legitimate' incident-specific characteristics (such as risk) that may correlate with geography but are not captured with the number of trees. The Street Tree data is available here: \url{https://data.cityofnewyork.us/Environment/2015-Street-Tree-Census-Tree-Data/pi5s-9p35}, and we use the same FCC API as before to convert lat/longs to census tracts.}

\end{figure}

 \begin{figure}[tb]
	\centering
%	\subfloat[][Reported incidents vs trees]{
		\includegraphics[width=.45\textwidth]{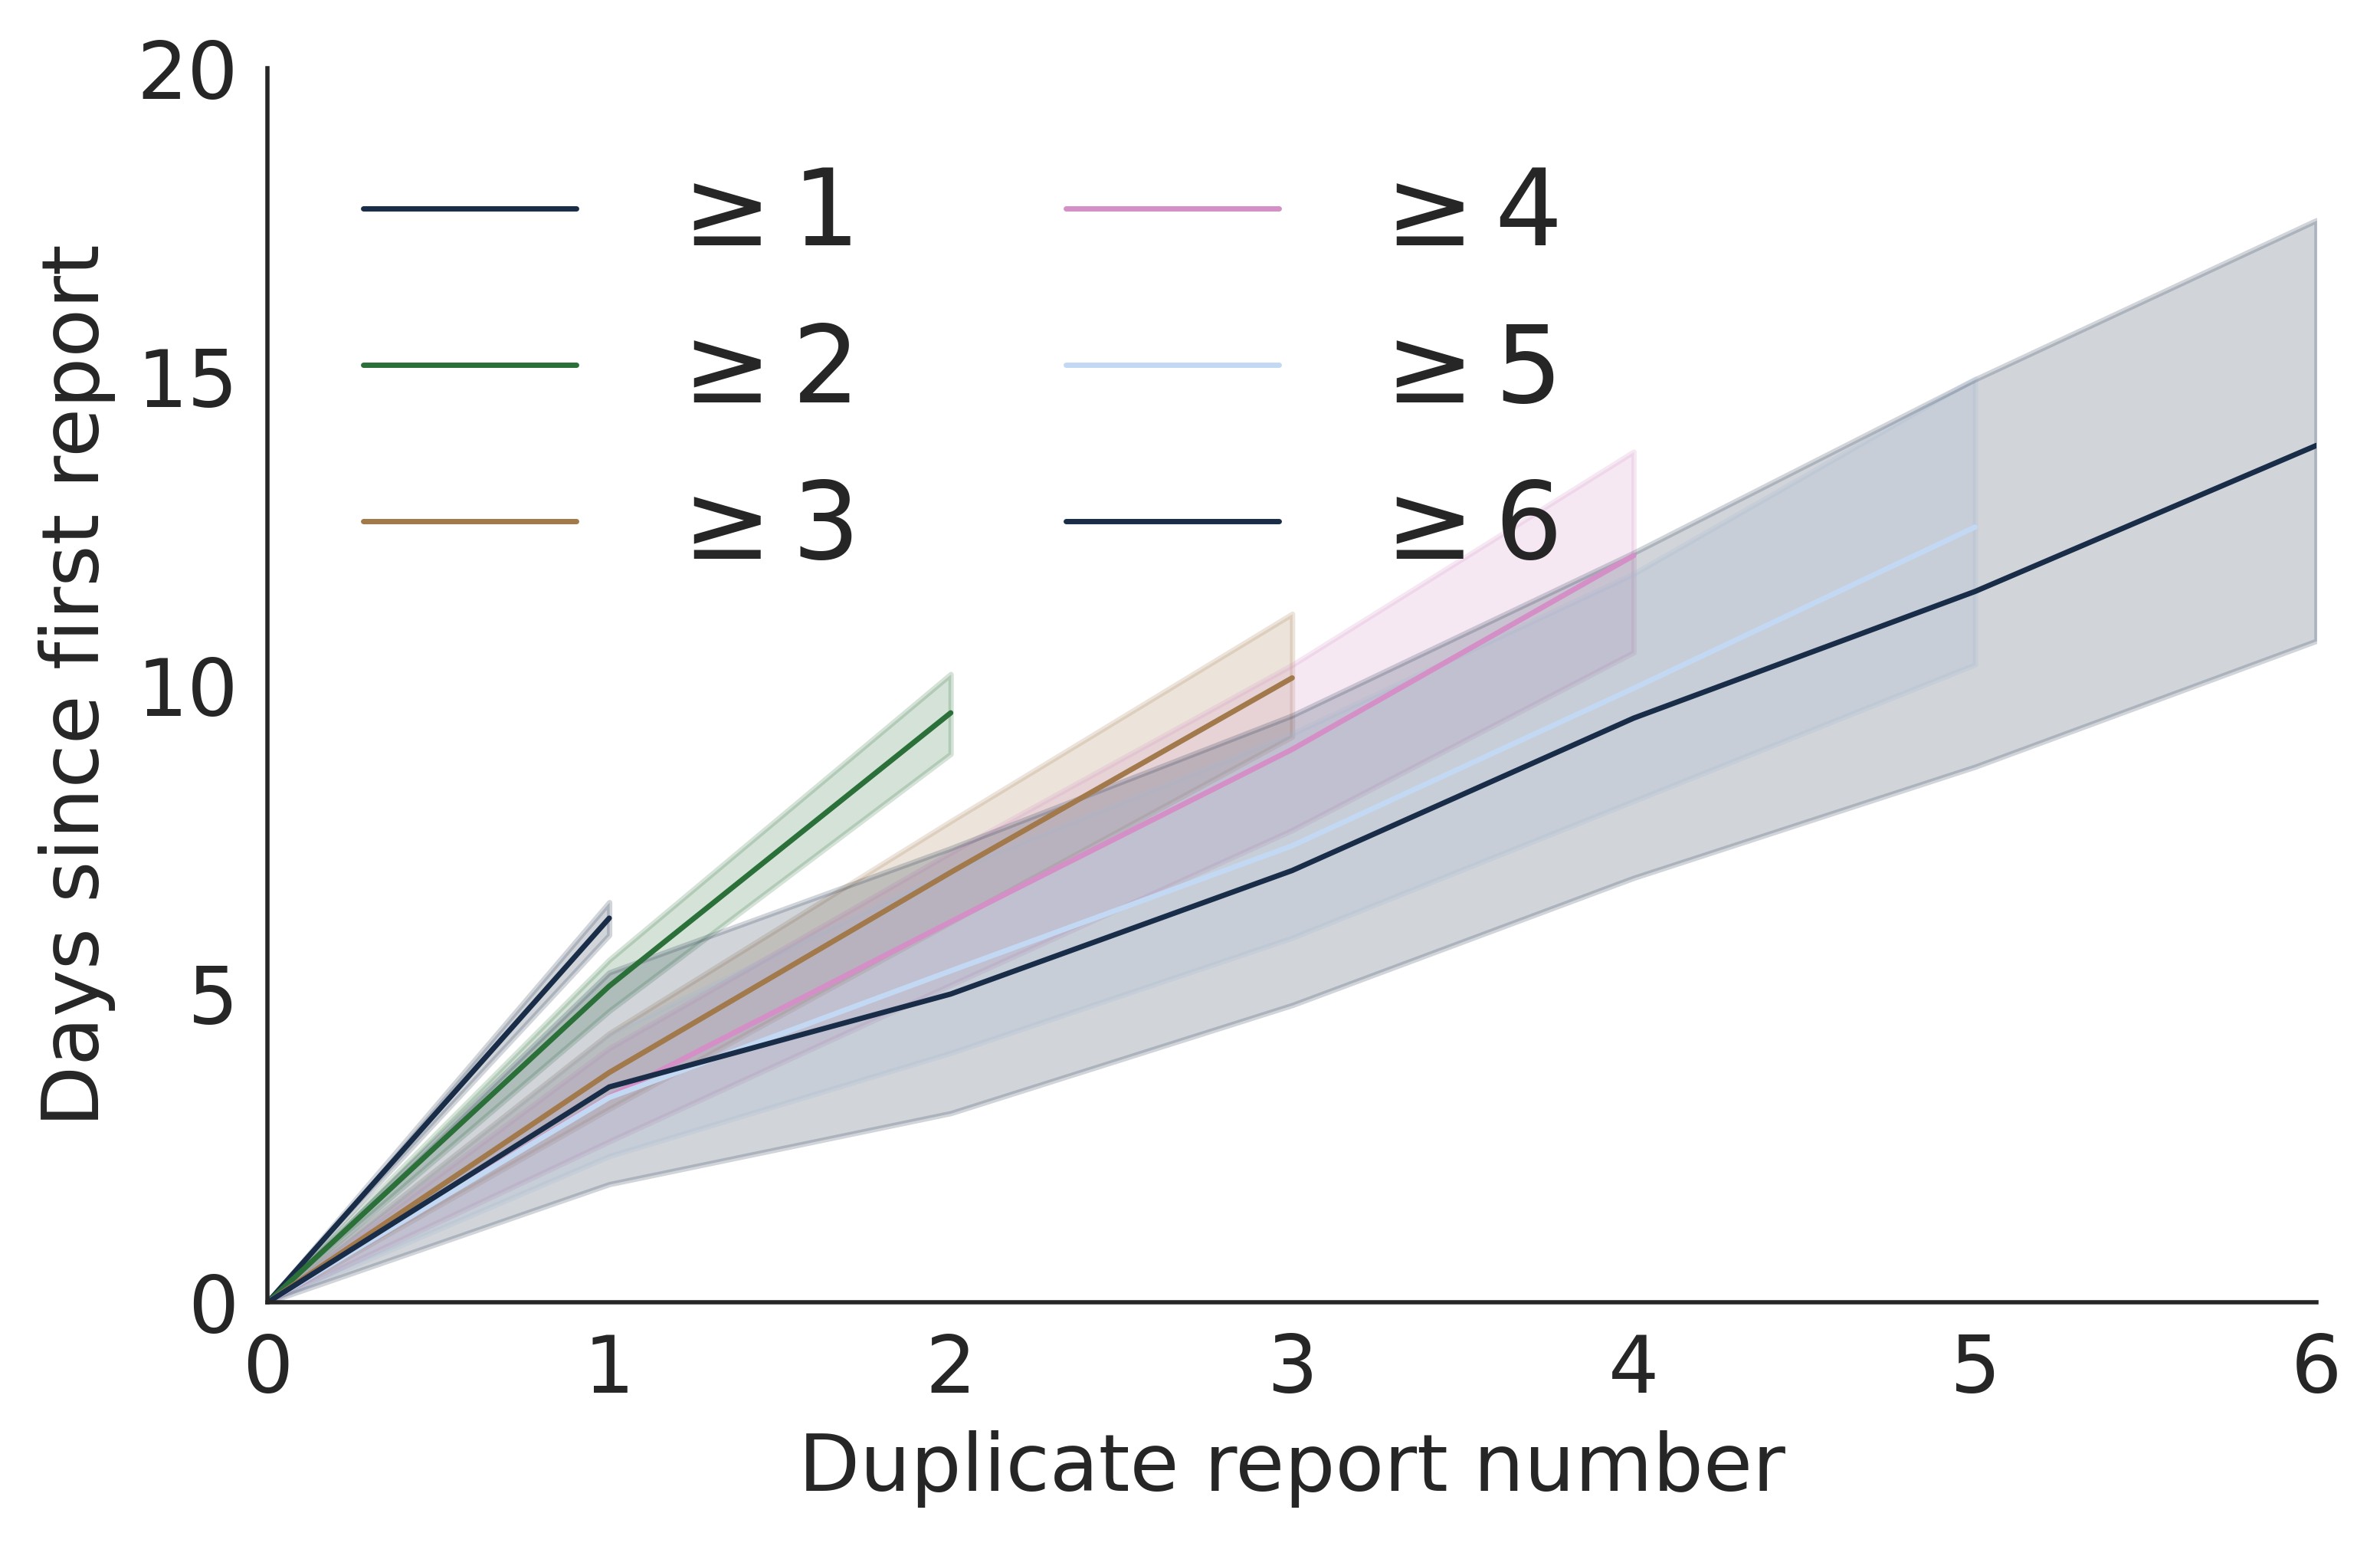}
%	}
%	\hfill
%	\subfloat[][Incidents/Tree vs Census Tract Coefficient]{
%		\includegraphics[width=.45\textwidth]{plots/incidents_per_tree_vs_coefficient}
%		\label{fig:reginccoef}
%	}
	\caption{Conditional on having at least $k$ duplicate reports, on average how many days after the $0th$ report was the $\ell$th report, where $\ell \leq k$? The linear nature of each plot is consistent with an homogeneous Poisson process within the given period. That incidents with more reports also receive reports \textit{faster} is consistent with those incidents being more severe in nature and having a higher reporting rate $\lambda_\theta$. }

			\label{fig:daysfirstcomplaint}
\end{figure}

 \begin{figure}[tb]
	\centering
	%	\begin{subfigure}{.5\textwidth}
	% 		\centering
	\subfloat[][Standard Poisson Regression]{
		\includegraphics[width=.45\textwidth]{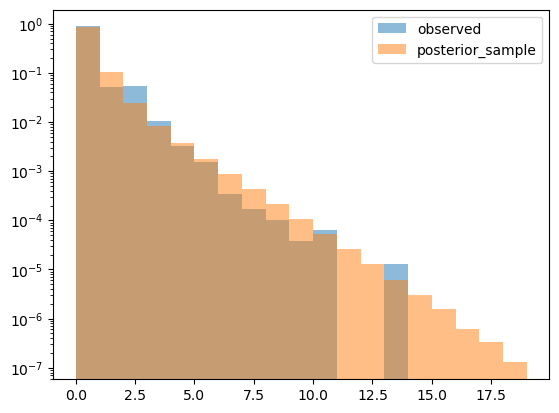}
%		\includegraphics[width=.45\textwidth]{plots/basic_nocens2_dur100_repmedium_300300-1nocens2_histograms.png}
		% 		\caption{Census tract fixed effects}
		\label{fig:basicposterior}
		% 		\end{subfigure}
	}
	\hfill
	\subfloat[][Zero inflated Poisson regression]{
				\includegraphics[width=.45\textwidth]{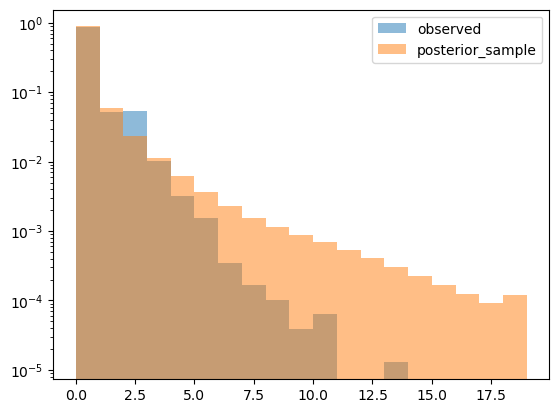}
%		\includegraphics[width=.45\textwidth]{plots/basic_zeroinflated_nocens2_dur100_repmedium_300300-1nocens2_histograms.png}
		% 		\caption{Census tract fixed effects}
		\label{fig:zifposterior}
		% 		\end{subfigure}
	}
	\caption{Comparison between posterior distributions sampled from the Standard Poisson regression model and the Zero-inflated variant. Note that the Zero-inflated model has a better fit to the observed distribution, since most of the density of this distribution is on reports 1, 2, and 3, even though the Standard model has a better fit for the higher values (the log scale may obscure some errors and amplify others).}
	\label{fig:posteriors}

\end{figure}

\input{plots/basic_zeroinflated_noborough_paper1_dur100_repmedium_300300-1singlecens2__unicoefsequity_full.tex}

\FloatBarrier
